# Supplementary material for: Optimal Transport for Domain Adaptation through Gaussian Mixture Models
Source: arXiv:2403.13847 source file (2025-07-08)
Supplement: Supplementary file 1 [file tables.tex]

\begin{table}[ht]
    \centering
    \begin{tabular}{ccccc}
        \toprule
        Benchmark                          & Domains         & Backbone                    & \# Samples & \# Classes           \\
        \midrule
        \multirow{4}{*}{ImageCLEF}         & Caltech (C)     & \multirow{4}{*}{ResNet 50}  & 600        & \multirow{4}{*}{12}  \\
                                           & Bing (B)        &                             & 600        &                      \\
                                           & ImageNet (I)    &                             & 600        &                      \\
                                           & Pascal (P)      &                             & 600        &                      \\
                                           & Total           &                             & 2400       &                      \\
        \midrule
        \multirow{4}{*}{Caltech-Office 10} & Amazon (A)      & \multirow{4}{*}{ResNet 101} & 958        & \multirow{4}{*}{10}  \\
                                           & dSLR (D)        &                             & 157        &                      \\
                                           & Webcam (W)      &                             & 295        &                      \\
                                           & Caltech (C)     &                             & 1123       &                      \\
                                           & Total           &                             & 2533       &                      \\
        \midrule
        \multirow{3}{*}{Office 31}         & Amazon (A)      & \multirow{3}{*}{Resnet 50}  & 2817       & \multirow{3}{*}{31}  \\
                                           & dSLR (D)        &                             & 498        &                      \\
                                           & Webcam (W)      &                             & 795        &                      \\
                                           & Total           &                             & 4110       &                      \\
        \midrule
        \multirow{4}{*}{Office-Home}       & Art (Ar)        & \multirow{4}{*}{ResNet 101} & 2427       & \multirow{4}{*}{65}  \\
                                           & Clipart (Cl)    &                             & 4365       &                      \\
                                           & Product (Pr)    &                             & 4439       &                      \\
                                           & Real World (Rw) &                             & 4357       &                      \\
                                           & Total           &                             & 15588      &                      \\
        \midrule
        \multirow{4}{*}{CWRU}              & 1772rpm (A)     & \multirow{4}{*}{MLP}        & 8000      & \multirow{4}{*}{10} \\
                                           & 1750rpm (B)     &                             & 8000      &                      \\
                                           & 1730rpm (C)     &                             & 8000      &                      \\
                                           & Total           &                             & 24000     &                      \\
        \bottomrule
    \end{tabular}
    \caption{Overview of Visual Domain Adaptation benchmarks}
    \label{tab:overview_benchmarks}
\end{table}

\begin{table}[ht]
    \centering
    \begin{tabular}{ccccc}
        \toprule
        Benchmark                          & Domains         & Backbone                    & \# Samples & \# Classes           \\
        \midrule
        \multirow{4}{*}{CWRU}              & 1772rpm (A)     & \multirow{4}{*}{MLP}        & 8000      & \multirow{4}{*}{10} \\
                                           & 1750rpm (B)     &                             & 8000      &                      \\
                                           & 1730rpm (C)     &                             & 8000      &                      \\
                                           & Total           &                             & 24000     &                      \\
        \midrule
        \multirow{6}{*}{TEP}              & Mode 1     & \multirow{6}{*}{Fully Convolutional}        & 2900      & \multirow{6}{*}{29} \\
                                           & Mode 2     &                             & 2845      &                      \\
                                           & Mode 3     &                             & 2899      &                      \\
                                           & Mode 4     &                             & 2865      &                      \\
                                           & Mode 5     &                             & 2883      &                      \\
                                           & Mode 6     &                             & 2897      &                      \\
                                           & Total           &                             & 17289     &                      \\
        \midrule
        \multirow{7}{*}{CSTR}              & $N=1.0, \epsilon=0.00$     & \multirow{7}{*}{-}        & 1300      & \multirow{7}{*}{13} \\
                                           & $N=1.0, \epsilon=0.10$     &                             & 260      &                      \\
                                           & $N=1.0, \epsilon=0.15$     &                             & 260      &                      \\
                                           & $N=0.5, \epsilon=0.15$     &                             & 260      &                      \\
                                           & $N=1.5, \epsilon=0.15$     &                             & 260      &                      \\
                                           & $N=2.0, \epsilon=0.15$     &                             & 260      &                      \\
                                           & Total           &                             & 2860     &                      \\
        \bottomrule
    \end{tabular}
    \caption{Overview of Cross-Domain Fault Diagnosis benchmarks}
    \label{tab:overview_benchmarks_cdfd}
\end{table}
